# Supplementary material for: Mobility-induced kinetic effects in multicomponent mixtures
Source: arXiv:2405.02159 source file (2024-05-03)
Supplement: Supplementary file 1 [file SM.pdf]

# Supplemental Material for Mobility-induced kinetic effects in multicomponent mixtures

Filipe C. Thewes,[1] Matthias Krüger,[1] and Peter Sollich[1,2]
[1]Institut für Theoretische Physik, Georg-August-Universität Göttingen, 37077 Göttingen, Germany
[2]King's College London, Department of Mathematics, Strand, London WC2R 2LS, U.K.

## 1. LATTICE GAS MOBILITY

Consider the Hamiltonian on the lattice

$$H = \sum_{\boldsymbol{x}\sim\boldsymbol{x}'} \sum_{i,j=1}^{M} n_i(\boldsymbol{x}) n_j(\boldsymbol{x}') \epsilon_{ij} \tag{S1}$$

as defined in the main text. A configuration at the discretized time $t$ is specified by the collection $\boldsymbol{N}_t = \{n(t)\}$. Using the Martin-Siggia-Rose approach, the dynamics of the lattice gas can be written in terms of the conditional probability of observing a state $\boldsymbol{N}_{t+\Delta t}$ at time $t+\Delta t$ given that a state $\boldsymbol{N}_t$ was observed at time $t$, that is [1]

$$P(\boldsymbol{N}_{t+\Delta t}|\boldsymbol{N}_t;\Delta t) \propto \int d\hat{\boldsymbol{N}}_t e^{i\hat{\boldsymbol{N}}_t(\boldsymbol{N}_{t+\Delta t}-\boldsymbol{N}_t)+\sum_p w_p(\boldsymbol{N}_t)\Delta t(e^{-i\hat{\boldsymbol{N}}_t\boldsymbol{Q}_p}-1)}, \tag{S2}$$

where $\boldsymbol{Q}_p$ is the stoichiometry of the process $p$ and $w_p$ the rate at which it occurs; $p$ labels all possible swaps of particles with neighboring particles or vacancies. The resulting action in the above expression can be expanded up to second order in the inverse of the linear system size $\ell$ once the diffusive hydrodynamic scaling $(\tilde{\boldsymbol{x}},\tilde{t}) = (\boldsymbol{x}/\ell, t/\ell^2)$ is introduced and the occupation variables are parameterized by $n_i(\boldsymbol{x},t) = 1$ with probability $\phi_i(\tilde{\boldsymbol{x}},\tilde{t})$ and $n_i(\boldsymbol{x},t) = 0$ with probability $1-\phi_i(\tilde{\boldsymbol{x}},\tilde{t})$. This yields the corresponding fluctuating hydrodynamics equation. If we consider jumps with Glauber-like acceptance rates $w^{ij}/(1+e^{\Delta H/T})$ for swapping the positions of particles of type $i$ and $j$, then in the limit $l\to\infty$ we can read off the current $\boldsymbol{j}_i$ of each species. After identifying the chemical potentials from the Flory free energy, the resulting mobility is found to be

$$L_{ij}(\boldsymbol{x}) = \frac{\phi_{\text{tot}}\sum_{k=0}^{M} w^{ik}\phi_k}{T}\left[c_i\delta_{ij} - \frac{\phi_{\text{tot}} w^{ij} c_i c_j}{\sum_{k=0}^{M} w^{ik}\phi_k}\right]. \tag{S3}$$

where the $w^{ij}$ are the rates at which neighboring particles of species $i$ and $j$ swap positions (Fig. S1). This is the mobility in Eq. (19) in the main text.

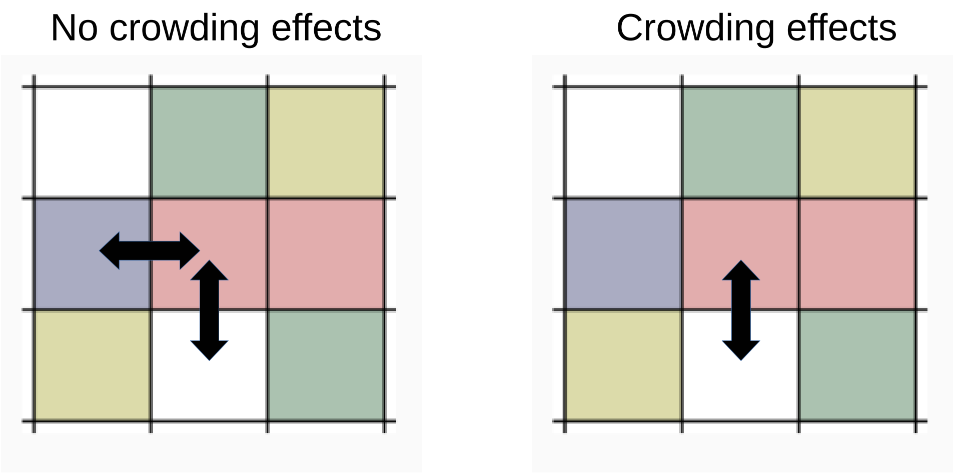


FIG. S1. Lattice gases with distinct underlying kinetic rules. On the left, neighboring particles of species $i$ and $j$ swap positions with rate $w^{ij}$. Similarly, a particle will swap positions with a neighboring vacancy at rate $w^{i0}$. On the right, $w^{ij} = 0$ for nonzero $i$ and $j$, and only swaps with vacancies are allowed. These different kinetic rules give rise to distinct mobilities.

## 2. EQUILIBRIUM INTERFACES AND COARSENING

We discuss in this section the issue of determining equilibrium interface profiles in multicomponent mixtures. Similarly to the task of finding the number and properties of coexisting bulk phases, this becomes a challenging question as the number of components increases. For the single component case, a detailed exposition can be found in [2, 3]. In the multicomponent case, equality of chemical potentials $\mu_i = \delta F/\delta\phi_i$ across an interface between two phases requires, for constant $\boldsymbol{K}$,

$$\boldsymbol{K}\nabla^2\boldsymbol{\phi} = \frac{\partial f_{\mathrm{bulk}}}{\partial\boldsymbol{\phi}} - \boldsymbol{\mu}. \tag{S4}$$

The shape of an interface between two phases therefore depends on the bulk free energy (in particular its curvature as one sees by linearizing the r.h.s. away from the interface) and the interfacial matrix $\boldsymbol{K}$. To determine the surface tension associated with an interface between phases $\alpha$ and $\gamma$ one can consider an interface orthogonal to one of the Cartesian directions, say $x_1$, and solve (S4) for $\boldsymbol{\phi}(x_1)$. Extending the derivation in [3, 4] we find the surface tension

$$\sigma_{\alpha\gamma} = \int dx_1\, V(\boldsymbol{\phi}(x_1)) = \int_{\boldsymbol{\phi}^\alpha}^{\boldsymbol{\phi}^\gamma} dl \sqrt{2V(\boldsymbol{\phi}(l))\frac{\partial_l\boldsymbol{\phi}^{\mathrm{T}}\boldsymbol{K}\partial_l\boldsymbol{\phi}}{\partial_l\boldsymbol{\phi}^{\mathrm{T}}\partial_l\boldsymbol{\phi}}}. \tag{S5}$$

where the second form is a line integral in $\boldsymbol{\phi}$-space. For a single component the known result [3] $\sigma = \int d\phi\sqrt{2KV(\phi)}$ is retrieved.

For curved interfaces that occur e.g. when a droplet of a given phase $\alpha$ is immersed in a sea of phase $\gamma$, one can proceed similarly [3]. Assuming that $\boldsymbol{\phi}$ depends only on $g$, the coordinate in the direction normal to the interface, Eq. (S4) becomes

$$\boldsymbol{\mu} = -\boldsymbol{K}\left(\frac{\partial^2\boldsymbol{\phi}}{\partial g^2} + \frac{\partial\boldsymbol{\phi}}{\partial g}\nabla\cdot\hat{\boldsymbol{g}}\right) + \frac{\partial f_{\mathrm{bulk}}}{\partial\boldsymbol{\phi}}. \tag{S6}$$

where $\hat{\boldsymbol{g}}$ is the unit vector along the gradient of $g$. Multiplying by $\partial\boldsymbol{\phi}^{\mathrm{T}}/\partial g$ on both sides and integrating over $g$ gives the Gibbs-Thomson boundary condition [3] in the multicomponent case

$$\boldsymbol{\mu}^{\mathrm{T}}\Delta\boldsymbol{\phi} = G\sigma_{\alpha\gamma} + \Delta f_{\mathrm{bulk}} \tag{S7}$$

where $G$ quantifies the interface curvature, e.g. $G = (d-1)/R$ for a spherical interface with radius $R$ in $d$ dimensions, and $\Delta\boldsymbol{\phi}$ and $\Delta f_{\mathrm{bulk}}$ indicate the differences between the values inside and outside the droplet, far from the interface. Given the common tangent relation for coexisting phases

$$V(\boldsymbol{\phi}) \equiv f_{\mathrm{bulk}}(\boldsymbol{\phi}) - \sum_i \mu_i\phi_i + \Pi = 0, \tag{S8}$$

Eq. (S7) can be written also as $\Delta\Pi = (d-1)\sigma_{\alpha\gamma}/R$, i.e. the pressure difference is just the Laplace pressure.

In order to obtain the time evolution of the boundary of a droplet, one makes use of the dynamical equation

$$\dot{\phi}_i(\boldsymbol{x},t) = \sum_j \nabla\cdot\left[\int d\boldsymbol{x}'\int_0^t dt' L_{ij}\left(\boldsymbol{x}-\boldsymbol{x}', t-t'\right)\nabla'\frac{\delta F}{\delta\phi_j}\right] + \sqrt{2T}\nabla\cdot\boldsymbol{\eta}_i(\boldsymbol{x},t). \tag{S9}$$

Assuming the composition of the phases adjust rapidly to the current position of the droplet boundary, Eq. (S9) implies that the chemical potentials must satisfy $\nabla\cdot(\boldsymbol{L}\nabla\boldsymbol{\mu}) = 0$ subject to the boundary condition (S7). For simplicity, we assume the mobility to be local in space and time so that the Laplace equation $\nabla^2\boldsymbol{\mu} = 0$ follows. One then has that the velocity $v = dR/dt$ of the domain wall is

$$\frac{\partial}{\partial t}\int dg\,\boldsymbol{\phi} = -v\Delta\boldsymbol{\phi} = \Delta\left(\boldsymbol{L}\frac{\partial\boldsymbol{\mu}}{\partial g}\right). \tag{S10}$$

Due to the Laplace equation, $\partial_g\boldsymbol{\mu}$ must be zero inside the droplet and the above expression reduces to $\boldsymbol{L}^\gamma\partial_g\boldsymbol{\mu} = -v\Delta\boldsymbol{\phi}$ where $\boldsymbol{L}^\gamma$ is the mobility evaluated in the outside ($\gamma$) phase.

Combining (S7) with (S10)then gives

$$\frac{dR}{dt} = \frac{2\sigma_{\alpha\gamma}}{R\Delta\boldsymbol{\phi}^{\mathrm{T}}(\boldsymbol{L}^\gamma)^{-1}\Delta\boldsymbol{\phi}}\left(\frac{1}{R_c} - \frac{1}{R}\right) \tag{S11}$$

with $R_c = 2\sigma_{\alpha\gamma}/\Delta\Pi$ the critical radius, as stated in the main text in Eq. (20).

---

[1] A. Lazarescu, T. Cossetto, G. Falasco, and M. Esposito, Large deviations and dynamical phase transitions in stochastic chemical networks, J. Chem. Phys. **151**, 10.1063/1.5111110 (2019).
[2] J. W. Cahn and J. E. Hilliard, Free energy of a nonuniform system. i. interfacial free energy, J. Chem. Phys. **28**, 258–267 (1958).
[3] A. J. Bray, Theory of phase-ordering kinetics, Adv. Phys. **43**, 357 (1994).
[4] G. Kaptay, On the interfacial energy of coherent interfaces, Acta Mater. **60**, 6804 (2012).
